# Supplementary material for: Multiple View Neural Regression of a Facial Shape Model
Source: arXiv:2608.22655 source file (2026-08-23)
Supplement: Supplementary file 1 [file appendixA.tex]

\section{Extra Cool Stuff}
This is often a good section to place additional specifics, how-to images, code, whatever... things that add detail to your thesis but might break-up reading the main document too much.


\begin{figure}
\begin{center}
\includegraphics{testbed}
\end{center}
\end{figure}
