# Supplementary material for: Multiple View Neural Regression of a Facial Shape Model
Source: arXiv:2608.22655 source file (2026-08-23)
Supplement: Supplementary file 2 [file appendixB.tex]

\section{More Cool Stuff}
Another addendum in a specific area such as any other appendices.
